# Supplementary material for: Sparse Cyclic Excitations Explain the Low Ionic Conductivity of Stoichiometric Li$_{7}$La$_{3}$Zr$_{2}$O$_{12}$
Source: arXiv:1511.08883 source file (2015-11-28)
Supplement: Supplementary file 1 [file SI.pdf]

# Supplemental Materials: Sparse Cyclic Excitations Explain the Low Ionic Conductivity of Stoichiometric $Li_7La_3Zr_2O_{12}$

## Li sublattice of LLZO

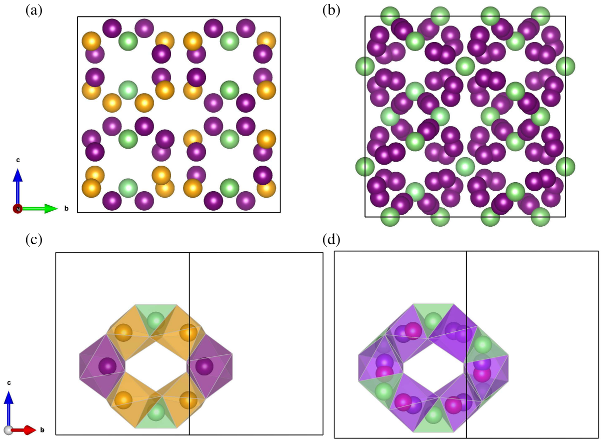


FIG. S1. Li positions in tetragonal (a) and cubic (b) LLZO. The green spheres correspond to tetrahedral sites in both systems, while yellow and purple represent octahedral sites. Panels (c) and (d) illustrate the 8-membered rings in the same sublattices as (a) and (b) viewed along the [110] axis.

## Extended excitation event

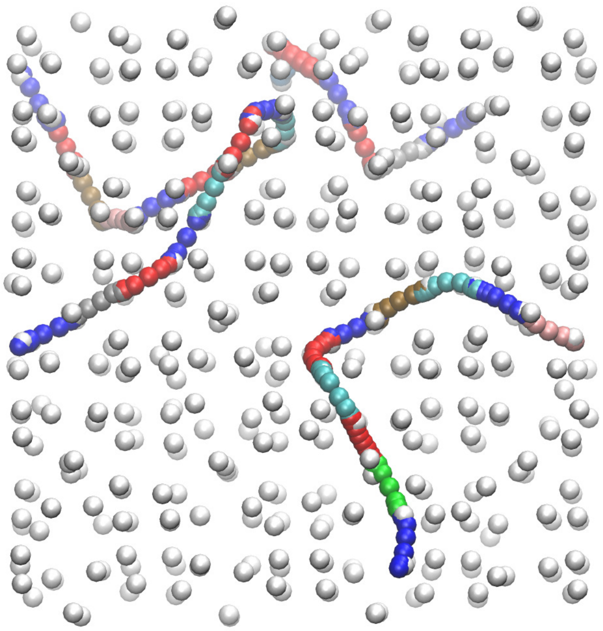

FIG. S2. Coalescent excitation event in LLZO at 300 K.

## Potential derivation

One of the most distinctive features of the IP parameterization methodology presented in this paper is that the parameters are derived entirely from *ab initio* data, with no direct input of experimentally measured properties. As such, it is crucial that the agreement between DFT and DIPPIM be as close as possible for the potential parameters to be accepted. Fig. S3 illustrates the results obtained for the fit for one of the LLZO configurations that were used. The fits included 3 LLZO unit cells with 192 atoms, of which 2 had tetragonal symmetry and 1 with cubic symmetry and which were set up by randomly distributing the lithiums over the tetrahedral and octahedral sites to achieve an occupancy ratio equal to that of Xu *et al.* [1], that is 43% of the Li ions occupy the tetrahedral positions and the rest were placed in the octahedral positions. The fit also included two Al-doped LLZO unit cells of compostions $Li_{4.0}Al_{1.0}La_3Zr_2O_{12}$ and $Li_{4.75}Al_{0.75}La_3Zr_2O_{12}$, one each of Nb-doped and Ta-doped LLZO with compositions $Li_{6.0}La_3ZrMO_{12}$, one each of $Li_5La_3Nb_2O_{12}$ and $Li_5La_3Ta_2O_{12}$, as well as, two 2×2×2 supercells of $LiAlO_2$. All dopant atoms were randomly placed in the LLZO cells, Al over the tetragonal Li sites in the cell, while Nb and Ta occupied Zr sites. Each panel presents the h-DFT values that were used for the fit as open black symbols, while those obtained using DIPPIM are shown as filled orange symbols. The top panel presents the forces along the $x$-axis for each ion in the order $O^{2-}$, $La^{3+}$, $Zr^{4+}$, $Li^{+}$. The middle panel presents the dipole moments along the $x$-axis for all the ions, except Li, which is considered to be non-polarizable. The bottom panel presents the stress tensor components. As is evident from these results, the DIPPIM potentials offer accuracies comparable to the hybrid-DFT from which they were derived while incurring a computational cost several orders of magnitude lower.

Each cell included in the fit was prepared using *ab initio* MD simulations at a temperature of 2000 K using the PBE functional[2] with a 300 eV plain wave cut-off, $k$-point sampling at the gamma point only and a timestep of 1 fs. The cells were equilibrated for approximately 50 ps in order to ensure that the forces on most ions were greater than $1\,\mathrm{eV}\,\mathrm{\AA}^{-1}$. Subsequent to the high temperature equilibrations, static h-DFT (HSE06 [3, 4]) calculations with a larger plane wave cut-off of 500 eV were performed to obtain reliable forces and stress tensors. The wavefunctions were then post-processed using the wannier90 library [5] and the resulting wannier centres were used to calculate the dipole moments on each ion. The parameters obtained thusly and employed

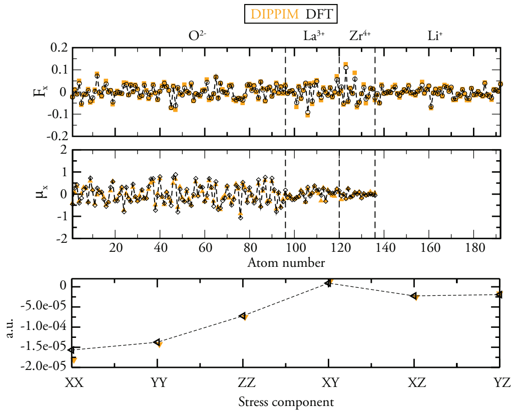


FIG. S3. DIPPIM (filled orange symbols) and h-DFT (open black symbols) calculated forces (top), dipole moments (middle) and stress tensors (bottom) in atomic units.

throughout this study are reported in Table S1. All *ab initio* simulations were performed using the VASP code.

The dipole polarizabilities for $La^{3+}$, $Zr^{4+}$ and $O^{2-}$ were obtained from previous work [6], while those for $Nb^{5+}$ $Ta^{5+}$ were included in the fit. In all cases, the dispersion terms were derived from these polarizabilities by means of the Slater-Kirkwood equation [6, 7].

### Simulation Details

All MD simulations on the lithium garnet $Li_7La_3Zr_2O_{12}$, were performed using $2 \times 2 \times 2$ supercells with 1536 atoms that were generated from the cells used to perform the potential parameterization (See below). The supercells were initially equilibrated at a temperature of 280 K for 10 ps; the temperature was then scaled up to 1000 K at a rate of $1\,\mathrm{K\,ps^{-1}}$ to study the changes in lattice constant as a function of temperature. All the equilibration simulations were performed at constant temperature and pressure (NPT ensemble), as described by Martyna *et al.* [8] using a time step of 1 fs. The Coulombic interactions were summed using Ewald summations [9], while the short-range part of the potential was truncated at 12.96 Å.

### Validation of the Interatomic Potential

The quality of the DIPPIM model was first assessed from its ability to accurately predict the structure and dynamics of LLZO, by performing a comparison with the available experimental data (for the structure) and DFT-based MD results (for the lithium diffusion).

The room temperature lattice constants obtained with DIPPIM are presented in Table S2 along with experimental and DFT literature values. The room temperature lattice parameters from the DIPPIM model are approximately 1% larger than experimental values, as would be expected due to the h-DFT functional used lacking dispersion interactions and also overestimating the volume. LLZO undergoes a phase transition from a tetragonal to cubic lattice at temperatures above 600 K. Experimental transition temperatures depend strongly on the incorporation of Al during sample preparation, and on exposure to air [12, 17]. The DIPPIM potential predicts a tetragonal (t-LLZO) crystal structure below 620 K and a cubic (c-LLZO) structure above 620 K (Fig. S4 (a)). This agrees with the experimental value of 623 K of Kuhn *et al.* , and with the value of 600 K from the DFT-based MD simulations of Bernstein *et al.* [18].

The calculated DIPPIM Li-Li partial radial distribution functions, $g(r)$, for t-LLZO at 300 K are presented in Fig. S4 (b) (green) along with those obtained by neutron scattering experiments (black) and the shell model from the work of Klenk and Lai [13]. The $g(r)$ from MD simulations using the soft bond-valence model of Adams and Rao [14] is shown in blue. The DIPPIM shows an excellent agreement with the experimental structure over the whole range of distances. Further confirmation that the DIPPIM model predicts the correct structure for LLZO was obtained by comparing the predicted fractional occupancies of the tetrahedral and octahedral sites as a function of temperature in t-LLZO with those obtained experimentally (Fig. S4 (d)). The experimental occupancy of the tetrahedral sites at room temperature obtained from NMR [12] is of 0.14, in excellent agreement with our simulated value of 0.15.

The DIPPIM predictions of Li-ion diffusivities were also validated with respect to the DFT-based MD values obtained at high-temperature by Miara *et al.* [15] (Fig. S4 (d)). The values span a range of 400–1000 K because no diffusion was observed at 300 K despite the long simulation time (87 ns). The slight overestimation by DIPPIM with respect to the DFT-based MD value is accounted for by the fact that Miara *et al.* constrained their simulation volumes to the smaller experimental values, which is equivalent to applying a negative isotropic strain to the system, which lowers the diffusivity with respect to its value at the equilibrium volume. The effects of strain in other ionic conductors have been widely explored in the literature [19, 20].


[1] M. Xu, M. S. Park, J. M. Lee, T. Y. Kim, Y. S. Park, and E. Ma, Phys. Rev. B **85**, 052301 (2012).
[2] J. P. Perdew, K. Burke, and Y. Wang, Physical Review B **54**, 16533 (1996).
[3] J. Heyd, G. E. Scuseria, and M. Ernzerhof, Journal of Chemical Physics **118**, 8207 (2003).
[4] J. Paier, M. Marsman, K. Hummer, G. Kresse, I. C. Gerber, and J. G. Angyan, The Journal of Chemical Physics

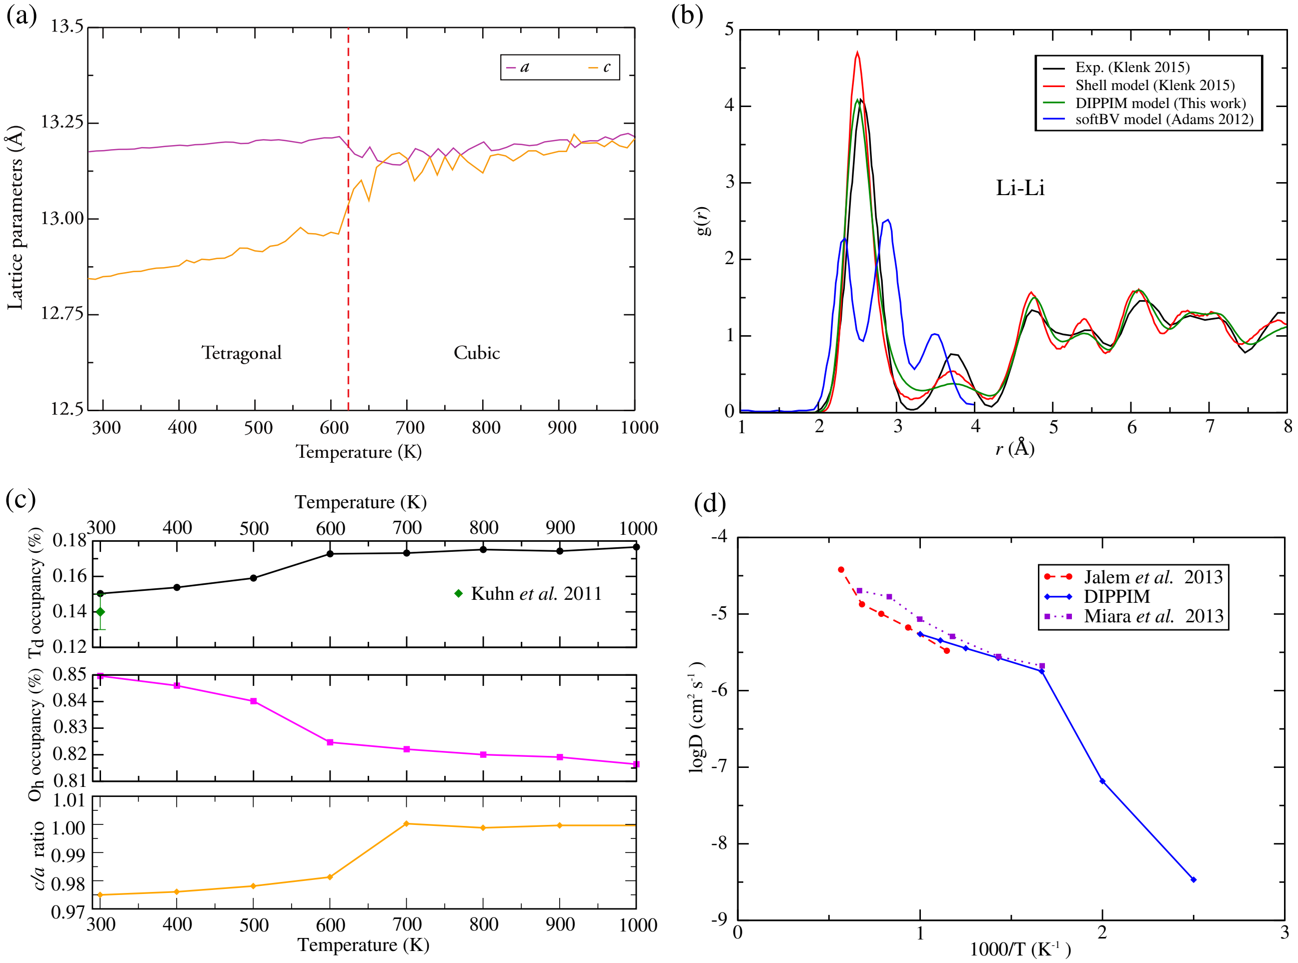


FIG. S4. (a) DIPPIM calculated lattice parameters (Å) for t-LLZO as a function of temperature (K) . The $a$ parameter is shown in magenta and the $c$ parameter is shown in orange. The red dashed line marks the transition temperature of 623 K found experimentally by Kuhn *et al.* [12] (b) Li-Li radial distribution function for t-LLZO from the work of Klenk and Lai [13] (Neutron scattering shown in black and shell model shown in red), as well as, Adams and Rao [14] (soft Bond Valence force field shown in blue). DIPPIM results are shown in green. (c) Occupancies of tetrahedral (top panel) and octahedral (middle panel) sites in pure LLZO as a function of temperature. The ratio of the $c/a$ vectors in the same temperature range is presented in the bottom panel. The tetrahedral occupancy at room temperature found by Kuhn *et al.* [12] using NMR expriments is shown as a green diamond in the top panel. (d) Diffusion coefficients for t-LLZO (blue diamonds). These values were calculated from the MSDs presented in Fig. 2 of the main text. The literature values correspond to the *ab initio* MD simulations from Miara *et al.* [15] (purple squares) and Jalem *et al.* [16] (red circles).

**124**, 154709 (2006).

[5] A. A. Mostofi, J. R. Yates, Y.-S. Lee, I. Souza, D. Vanderbilt, and N. Marzari, Computer Physics Communications **178**, 685 (2008).

[6] M. Burbano, S. Nadin, D. Marrocchelli, M. Salanne, and G. W. Watson, Phys. Chem. Chem. Phys. **16**, 8320 (2014).

[7] J. C. Slater and J. G. Kirkwood, Physical Review **37**, 682 (1931).

[8] G. J. Martyna, D. J. Tobias, and M. L. Klein, Journal of Chemical Physics **101**, 4177 (1994).

[9] P. P. Ewald, Annalen der Physik **369**, 253 (1921).

[10] E. Rangasamy, J. Wolfenstine, J. Allen, and J. Sakamoto, Journal of Power Sources **230**, 261 (2013).

[11] K. Meier, T. Laino, and A. Curioni, J. Phys. Chem. C **118**, 6668 (2014).

[12] A. Kuhn, S. Narayanan, L. Spencer, G. Goward, V. Thangadurai, and M. Wilkening, Phys. Rev. B **83**, 094302 (2011).

[13] M. Klenk and W. Lai, Phys. Chem. Chem. Phys. (2015), 10.1039/C4CP05690F.

[14] S. Adams and R. P. Rao, J. Mater. Chem. **22**, 1426 (2011).

[15] L. J. Miara, S. P. Ong, Y. Mo, W. D. Richards, Y. Park, J.-M. Lee, H. S. Lee, and G. Ceder, Chemistry of Materials **25**, 3048 (2013), http://pubs.acs.org/doi/pdf/10.1021/cm401232r.

[16] R. Jalem, Y. Yamamoto, H. Shiiba, M. Nakayama, H. Munakata, T. Kasuga, and K. Kanamura, Chem. Mater. **25**, 425 (2013).

[17] G. Larraz, A. Orera, and M. L. Sanjuan, J. Mater. Chem. A **1**, 11419 (2013).

[18] N. Bernstein, M. Johannes, and K. Hoang, Phys. Rev. Lett. **109**, 205702 (2012).
[19] M. Burbano, D. Marrocchelli, and G. Watson, Journal of Electroceramics **32**, 28 (2013).
[20] A. Kushima and B. Yildiz, Journal of Materials Chemistry **20**, 4809 (2010).

TABLE S1. Parameters for the DIPPIM potential. All values are in atomic units. The parameters $b_D^{O^{2-},\square}$ and $b_D^{\square,O^{2-}}$ were given the same value. $\square$ is a placeholder for the identity of the ionic species specified in a given column

| Interaction | $A^{ij}$ | $a^{ij}$ | $B^{ij}$ | $b^{ij}$ | $C_6^{ij}$ | $C_8^{ij}$ | $b_6^{ij}$ | $b_8^{ij}$ |
|---|---|---|---|---|---|---|---|---|
| $O^{2-} - O^{2-}$ | 0.00 | 5.00 | 50000 | 0.95 | 83.0 | 1240.0 | 1.30 | 1.70 |
| $Zr^{4+} - O^{2-}$ | 70.58 | 1.21 | 50000 | 1.75 | 21.0 | 271.0 | 1.62 | 2.10 |
| $La^{3+} - O^{2-}$ | 103.48 | 1.27 | 50000 | 1.30 | 57.0 | 731.0 | 1.46 | 1.88 |
| $Li^{1+} - O^{2-}$ | 20.29 | 1.39 | 50000 | 2.06 | 0.00 | 0.00 | – | – |
| $Al^{3+} - O^{2-}$ | 40.04 | 1.26 | 50000 | 2.10 | 0.00 | 0.00 | – | – |
| $Nb^{5+} - O^{2-}$ | 58.15 | 1.12 | 50000 | 1.80 | 17.6 | 224.8 | 1.86 | 2.42 |
| $Ta^{5+} - O^{2-}$ | 58.14 | 1.12 | 50000 | 1.80 | 17.4 | 222.3 | 1.86 | 2.42 |

| Ion | $\alpha$ | $b_D^{O^{2-} - \square}$ | $c_D^{O^{2-} - \square}$ | $c_D^{\square - O^{2-}}$ |
|---|---|---|---|---|
| $O^{2-}$ | 13.97 | 2.11 | 2.86 | – |
| $Zr^{4+}$ | 2.38 | 1.74 | 1.60 | -0.75 |
| $La^{3+}$ | 7.51 | 1.72 | 2.09 | 0.03 |
| $Li^{1+}$ | – | 1.82 | 1.42 | – |
| $Al^{3+}$ | – | 1.80 | 1.41 | – |
| $Nb^{5+}$ | 1.97 | 1.80 | 1.46 | -0.91 |
| $Ta^{5+}$ | 1.88 | 1.79 | 1.57 | -0.55 |

TABLE S2. Experimental and calculated lattice constants for t-LLZO at 300 K.

| Source | | $a$ (Å) | $c$ (Å) |
|---|---|---|---|
| XRD | Rangasamy *et al.* [10] | 13.068 | 12.702 |
| DFT (PBE functional) | Meier *et al.* [11] | 13.208 | 12.659 |
| DIPPIM | this work | 13.180 | 12.849 |
